# Supplementary material for: X-SCITLDR: Cross-Lingual Extreme Summarization of Scholarly Documents
Source: arXiv:2205.15051 source file (2022-05-30)
Supplement: Supplementary file 1 [file 8-appendix.tex]

\section*{Appendix}
\label{sec:appendix}

In this section, we present a list of hyperparameters picked by grid search in Tabel \ref{ta:hparam}.

\begin{table*}
\centering
\begin{tabular}{|c|l|r|r|r|r|} 
\hline
\multicolumn{1}{|l|}{Lang} & Type & \multicolumn{1}{l|}{lr} & \multicolumn{1}{l|}{seed} & \multicolumn{1}{l|}{N of beams} & \multicolumn{1}{l|}{repetition penalty} \\ 
\hline
EN & pipeline & 1.00E-05 & 1122 & 3 & 0.8 \\ 
\hline
\multirow{3}{*}{JA} & no intermediate & 1.00E-05 & 1122 & 2 & 1.00 \\ 
\cline{2-6}
 & task-intermediate & 3.00E-05 & 1122 & 2 & 1.00 \\ 
\cline{2-6}
 & language-intermediate & 1.00E-05 & 1122 & 2 & 1.00 \\ 
\hline
\multirow{3}{*}{DE} & no intermediate & 1.00E-05 & 1122 & 2 & 1.00 \\ 
\cline{2-6}
 & task-intermediate & 1.00E-05 & 1122 & 2 & 1.00 \\ 
\cline{2-6}
 & language-intermediate & 1.00E-05 & 1122 & 2 & 1.00 \\ 
\hline
\multirow{3}{*}{IT} & no intermediate & 1.00E-05 & 1122 & 3 & 1.00 \\ 
\cline{2-6}
 & task-intermediate & 1.00E-05 & 1122 & 3 & 1.00 \\ 
\cline{2-6}
 & language-intermediate & 1.00E-05 & 22 & 3 & 0.8 \\ 
\hline
\multirow{3}{*}{ZH} & no intermediate & 1.00E-05 & 22 & 3 & 0.8 \\ 
\cline{2-6}
 & task-intermediate & 1.00E-05 & 22 & 3 & 0.8 \\ 
\cline{2-6}
 & language-intermediate & 1.00E-05 & 22 & 3 & 0.8 \\
\hline
\end{tabular}
\caption{Hyperparameters determined on validation dataset for each setup.}
\label{ta:hparam}
\end{table*}
